# Supplementary material for: Production Rate Measurement of Tritium and Other Cosmogenic Isotopes in Germanium with CDMSlite
Source: arXiv:1806.07043 ancillary file (2019-08-16)
Supplement: Supplementary file 1 [file CDMSlite_R2_extended_DataRelease.pdf]

# CDMSlite Run 2 Data Release for Measurement of Cosmogenic Production Rates

SuperCDMS Collaboration

This document describes the extended public data release of CDMSlite Run 2 data and the use of these data in measuring cosmogenic production rates of  $^{68}\text{Ge}$ ,  $^{65}\text{Zn}$ ,  $^{55}\text{Fe}$ , and  $^3\text{H}$ . The rates determined using these data can be found in the associated paper [1]. Questions about the data or the extracted production rates should be directed to [supercdms-publications@fnal.gov](mailto:supercdms-publications@fnal.gov).

## 1 Description of Data

There are four text files accompanying this data release. They are located in the `data_files` directory of the `.zip` file.

**eventTime\_and\_Energy.txt:** This file consists of two columns of event information, sorted by increasing time. The first is the event time in days since the first event of this data set; the second is the event energy in  $\text{keV}_{ee}$  (details about the energy scale are described in [2] and the accompanying data release). The 2378 events included in this list are all single-scatter events (for the definition of this term see [1]) inside the fiducial volume that pass all data quality selection criteria and have a reconstructed energy of less than  $20 \text{ keV}_{ee}$ . The event energy spectrum is shown in Figure 1.

**efficiency.txt:** This file contains information on the energy-dependent efficiency function. The first of four columns corresponds to the energy in  $\text{keV}_{ee}$ . The second column gives the detection efficiency at that energy, and the third and fourth columns give the lower and upper  $1\sigma$  (68%) uncertainties on the efficiency, respectively. The uncertainties are given as the difference from the central efficiency. The efficiency is given from 0 to  $20 \text{ keV}_{ee}$ , and is shown in Figure 2.

**LivetimeFunction.txt:** The two columns in this file describe the (differential) live-time as function of calendar time in days. The first column is the time in days since the first event of this data set, and the second column gives the fraction of time on that particular day that the data acquisition was live. This value is zero for days where no data were acquired or where all data were removed by data quality cuts. Figure 3 shows a scatter plot of event energy vs. time and the live-time per day with the same time axis.

**Tritium\_and\_Compton.txt:** This file provides the probability distribution functions (PDFs) of the tritium spectrum and the Compton background used in the fit. The CDMSlite Run 2 resolution model (see [2]) has been applied to each PDF, but not the energy efficiency (from `efficiency.txt`). The first column gives the energy in  $\text{keV}_{ee}$  (the same as in `efficiency.txt`), and the tritium and Compton PDFs are given in the second and third columns, respectively.

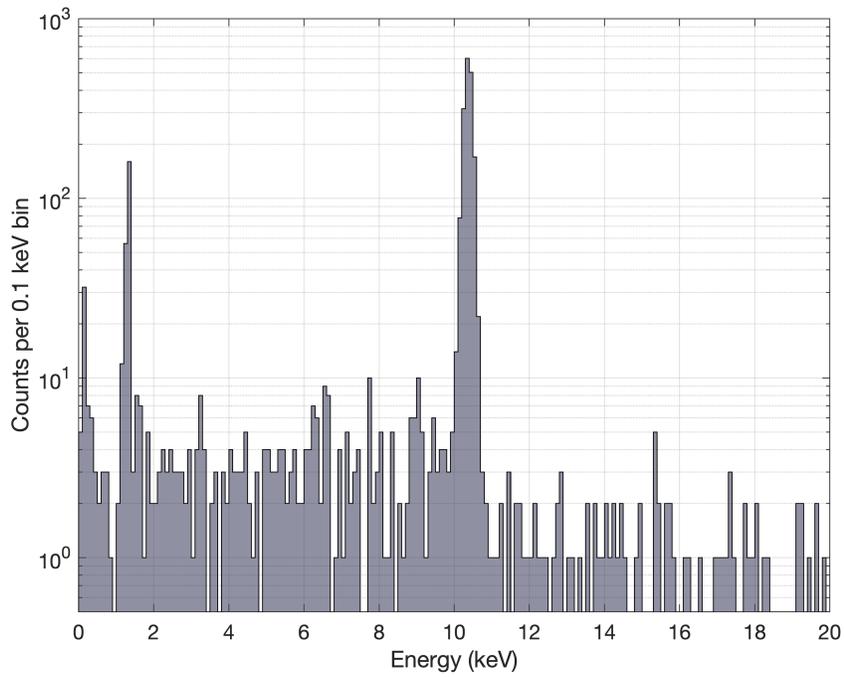

Figure 1: The CDMSlite Run 2 event spectrum from 0 to 20 keV<sub>ee</sub>. Events are from the second column of *eventTime\_and\_Energy.txt*.

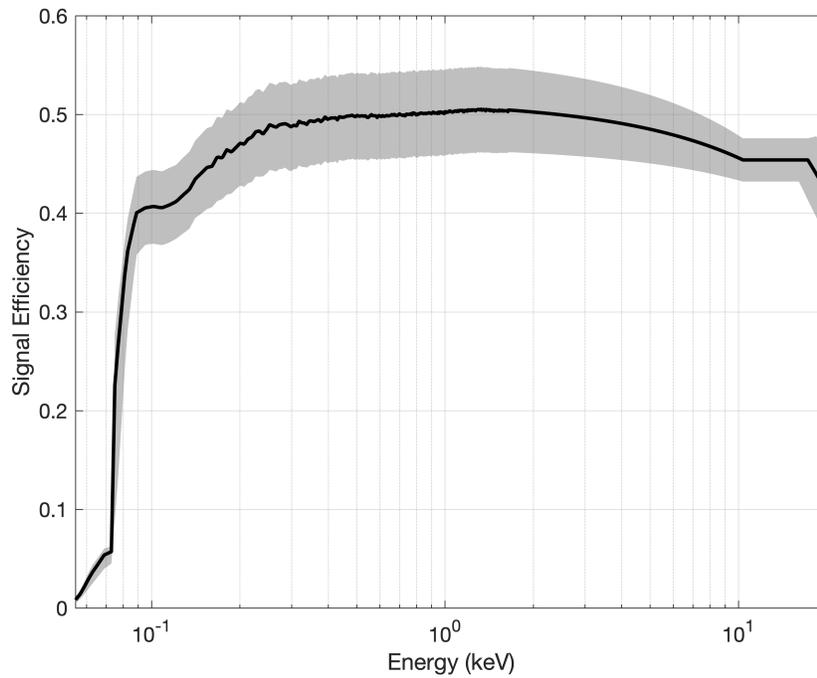

Figure 2: The CDMSlite Run 2 signal efficiency (black line) from 0 to 20 keV<sub>ee</sub>, with 1σ uncertainty band (grey), from *efficiency.txt*.

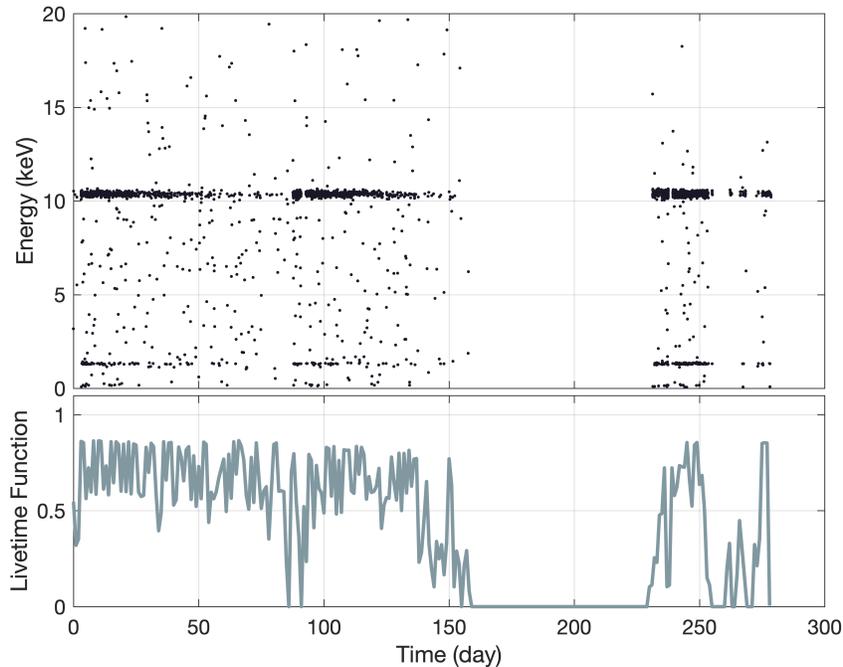

Figure 3: Event energy as a function of time (points) and differential live-time function (line).

## 2 Likelihood Fit

As described in the paper, the CDMSlite Run 2 spectrum is modelled by 9 backgrounds: tritium, Compton events, and electron capture (EC) backgrounds from  $^{68,71}\text{Ge}$ ,  $^{68}\text{Ga}$ ,  $^{65}\text{Zn}$ ,  $^{55}\text{Fe}$ ,  $^{58,57,56}\text{Co}$ ,  $^{54}\text{Mn}$ , and  $^{49}\text{V}$ . A likelihood fit is used to extract the contribution of each background. The tritium and Compton PDFs are given in `Tritium_and_Compton.txt`. The remaining 7 backgrounds are EC X-ray/ Auger electron peaks; their PDFs are modelled as Gaussian functions centred on the K-, L<sub>1</sub>-, and M<sub>1</sub>-shell binding energies of the daughter isotope. The resolution is set by the energy-dependent resolution model described in [2]. For an isotope with daughter isotope binding energies  $E_K$ ,  $E_{L_1}$ , and  $E_{M_1}$  for the K-, L<sub>1</sub>-, and M<sub>1</sub>-shells, the PDF is modelled as

$$\begin{aligned}
 f(E) = & \frac{P_K}{\sqrt{2\pi}\sigma_K} \exp\left(-\frac{(E - E_K)^2}{2\sigma_K^2}\right) \\
 & + \frac{P_{L_1}}{\sqrt{2\pi}\sigma_{L_1}} \exp\left(-\frac{(E - E_{L_1})^2}{2\sigma_{L_1}^2}\right) \\
 & + \frac{P_{M_1}}{\sqrt{2\pi}\sigma_{M_1}} \exp\left(-\frac{(E - E_{M_1})^2}{2\sigma_{M_1}^2}\right), \quad (1)
 \end{aligned}$$

where the  $P_X$  is the probability to capture an electron from the  $X$ -shell and  $\sigma_X$  is the resolution at  $E_X$ .  $E_X$ ,  $\sigma_X$ , and  $P_X$  can be found in Table 3 of the paper. The L<sub>2</sub>- and M<sub>2</sub>-shells are neglected

due to their small branching ratios ( $< \mathcal{O}(0.1\%)$ ) for all but Ge, where the  $L_2$  shell is included:

$$f(E) = \frac{P_K}{\sqrt{2\pi}\sigma_K} \exp\left(-\frac{(E - E_K)^2}{2\sigma_K^2}\right) + \frac{P_{L_1}}{\sqrt{2\pi}\sigma_{L_1}} \exp\left(-\frac{(E - E_{L_1})^2}{2\sigma_{L_1}^2}\right) + \frac{P_{L_2}}{\sqrt{2\pi}\sigma_{L_2}} \exp\left(-\frac{(E - E_{L_2})^2}{2\sigma_{L_2}^2}\right) + \frac{P_{M_1}}{\sqrt{2\pi}\sigma_{M_1}} \exp\left(-\frac{(E - E_{M_1})^2}{2\sigma_{M_1}^2}\right). \quad (2)$$

The energy dependent efficiency from `efficiency.txt` is then applied to each PDF, and the resulting functions are renormalized to PDFs that can be used in the likelihood fit.

These PDFs, denoted  $f_b(E)$  for background  $b$ , are then used to minimize the negative log-likelihood function with estimators  $n_b$ , the number of events that background  $b$  contributes. For the event energies in `eventTime_and_Energy.txt`, denoted  $E_i$  (where  $i = 1, \dots, 2378$ ), the negative log-likelihood function is

$$-\ln(\mathcal{L}) = \sum_b n_b - \sum_{i=1}^{2378} \ln\left(\sum_b n_b f_b(E_i)\right) \quad (3)$$

Uncertainties on the results of the likelihood fit are extracted from the one-dimensional likelihood as a function of number of events for the selected background. The distributions are found by fixing the number of events of a given background and calculating the maximum likelihood while allowing all other backgrounds to float. This process is repeated over an appropriate range. Normalizing to a PDF and converting to a cumulative distribution function (CDF) allows extraction of uncertainties at the desired level. Normalization is performed over the range 193.2 – 2378 events for Ge, 2.15 – 107.4 events for Zn, 27.0 – 1349.8 for H, 13.1 – 654.8 events for Compton, and -10 – 60 events for the remaining backgrounds. The negative event range accounts for when the uncertainty is larger than the absolute number of events.

### 3 Extracting Production Rates

The production rates are extracted in three steps:

- 1. Determine total number of decays in the detector:** The likelihood fit estimates the number of events that a background contributes to the measured spectrum, but due to the less than 100% signal efficiency this does not represent the total number of decays that occurred during the data taking period. Furthermore, not all decay modes are considered in the fit. For background  $b$ , the number of events extracted by the fit,  $N_b$ , must be converted to the total number of decays.  $N_b$  is scaled by an appropriate efficiency factor,  $R_{eff}$ , equal to 1 divided by the area of the background PDF with the efficiency function applied. This factor is approximately equal to 2 due to the  $\sim 50\%$  efficiency. The result is then divided by the branching ratio to the decay mode that the PDF describes. For example, the total number of events for tritium is

$$N_{3\text{H},total} = \frac{N_{3\text{H}} \cdot R_{eff}}{BR_{\beta^-}} = 265 \cdot 2.0732 \cdot 1 = 549.4. \quad (4)$$

Note that for  $^{65}\text{Zn}$  and  $^{68}\text{Ga}$ , which can decay via EC to an excited state, it is possible that the accompanying gamma can escape all of the detectors without interacting. As described

in the paper, this results in the event occurring in the singles peak. Therefore, instead of dividing by the EC ground state branching ratio, we have to divide by the effective efficiency, e.g. the probability that the event from a decaying Zn or Ga nucleus is reconstructed with an energy within the range of the respective EC peaks. This is  $(64.3 \pm 0.1)\%$  for  $^{65}\text{Zn}$  and  $(9.64 \pm 0.04)\%$  for  $^{68}\text{Ga}$ .

- 2. Determine the activity at the start of the run:** The activity of a given isotope, with decay constant  $\lambda$ , in the absence of production is  $A(t) = \frac{dN}{dt} = -\lambda N$ . The decay constant for each isotope relevant for this analysis can be determined from the corresponding half life, as given in Table 1 of the paper (note that  $\lambda = \ln 2/t_{1/2}$ , where  $t_{1/2}$  is the half life). The number of atoms of a given isotope in the detector at time  $t$  (in days) is  $N_0 \exp(-\lambda t)$ , where  $N_0$  is the number of atoms at the start of the run ( $t = 0$ ). To account for the live time of the detector, this is multiplied by the live time function from `LivetimeFunction.txt`,  $s(t)$ . The resulting function is normalized to 1. Multiplying by the total number of decays of the isotope, (determined in step 1) and dividing by the detector mass ( $m = 0.6065$  kg) gives the event rate as a function of time. The activity at  $t = 0$  is then this function evaluated at  $t = 0$  and divided by  $s(0)$ .

$$A(0) = \frac{N_{total} \exp(-\lambda t) s(t)}{m s(0) \int_0^{278.6} \exp(-\lambda t) s(t) dt} \Big|_{t=0} = \frac{N_{total}}{m \int_0^{278.6} \exp(-\lambda t) s(t) dt} \quad (5)$$

- 3. Solve for the production rate:** Using the detector history and the activity at the start of the run, the production rate can be determined. The detector location as a function of time since the crystal was pulled (is given in Table 1. The run start, at 1898 days, corresponds to  $t = 0$  in the event time data. Times in the table indicate when the detector changes location, i.e. on day 49 the detector was brought from the surface (S) to the underground (U) storage tunnel, where it remained until day 59 when it was brought back to the surface.

|             |     |     |     |        |     |     |     |      |           |     |
|-------------|-----|-----|-----|--------|-----|-----|-----|------|-----------|-----|
| Time (days) | 0   | 49  | 59  | 121±30 | 210 | 309 | 315 | 317  | 333       | 347 |
| Location    | S   | U   | S   | U      | S   | U   | S   | U    | S         | U   |
| Time (days) | 366 | 434 | 438 | 497    | 498 | 791 | 829 | 1065 | 1898      |     |
| Location    | S   | U   | S   | U      | S   | U   | S   | M    | Run Start |     |

Table 1: Detector location as a function of time in days from crystal pulling. Locations are S - surface (full exposure), U - underground (no exposure), M - Soudan mine (no exposure). Data taking started 1898 days after the crystal was pulled. The value  $121 \pm 30$  corresponds to uncertainty in the detector history logs.

During periods when the detector was above ground, the change in abundance is

$$\frac{dN}{dt} = P - \lambda N, \quad (6)$$

where  $P$  is the production rate. Similarly, during periods when the detector was underground, the change in abundance is

$$\frac{dN}{dt} = -\lambda N. \quad (7)$$

Using equation 6, the number of atoms per kg,  $N_U$  at time  $t_U$  when the detector is brought underground is

$$N_U = \left(N_S - \frac{P}{\lambda}\right) \exp(-\lambda(t_U - t_S)) + \frac{P}{\lambda} \quad (8)$$

where  $t_S$  is the time when the detector was previously brought to the surface and  $N_S$  is the number of atoms per kg at time  $t_S$ . The number of atoms,  $N_S$  at a time  $t_S$  when the detector is brought to the surface is found using equation 7:

$$N_S = N_U \exp(-\lambda(t_U - t_S)). \quad (9)$$

Starting with  $N_S = 0$  for  $t_S = 0$ , one can express  $N_0$ , the number of atoms per kg at the beginning of the run, as a function of  $P$ . As the detector was underground for the run, the activity at this point is  $-\lambda N_0$ . Using the activity determined in step 2 and equating to  $-\lambda N_0$  (where  $N_0$  is expressed in terms of  $P$ ), one can then solve for the production rate.

The uncertainty on the production rate from the uncertainty on the date that the detector was brought underground,  $121 \pm 30$  in Table 1, is determined by calculating the production rate using the extreme values, 91 and 151. The difference from the production rate using the central value is propagated into the final uncertainty.

## References

- [1] R. Agnese et al. (SuperCDMS Collaboration), Production rate measurement of tritium and other cosmogenic isotopes in germanium with CDMSlite, *Astropart. Phys.* 104 (2019) 1–12. doi:10.1016/j.astropartphys.2018.08.006.
- [2] R. Agnese et al. (SuperCDMS Collaboration), WIMP-search results from the second CDMSlite run, *Phys. Rev. Lett.* 116 (2016) 071301. doi:10.1103/PhysRevLett.116.071301.
